# Supplementary material for: A Nonparametric Frequency Domain EM Algorithm for Time Series Classification with Applications to Spike Sorting and Macro-Economics
Source: arXiv:1103.3300 source file (2011-10-02)
Supplement: Supplementary file 1 [file appendix.tex]

\section{KL divergence and MLE}
The Kullback-Leibler (KL) divergence between two discrete probability distribution $p_1, \ldots, p_K$ and $q_1, \ldots, q_K$ is defined as
\begin{equation}
\KL{p}{q} := \sum_{i=1}^{K} p_i \logtwo \frac{p_i}{q_i}  = \E_p \logtwo \frac{p_i}{q_i}.
\end{equation}
For the continuous case
\begin{equation}
\KL{p}{q} := \int p(x) \log \frac{p(x)}{q(x)} dx,
\end{equation}
where $p(x)$ and $q(x)$ are probability density functions.

KL divergence measures how far $p$ and $q$ are apart. In particular, note that if $p = q$ then $\KL{p}{q} = 0$; and if $p$ and $q$ are independent (or more precisely their RVs) then $\KL{p}{q} = \infty$. Note however, that in general KL divergence is not symmetric: $\KL{p}{q} \neq \KL{q}{p}$. From the definiton it is intuitive that the second argument is typically a reference/``true'' value, whereas the first argument is the one we want to see how far it is from that reference distribution.

Let $\tilde{p}(x)$ be the empirical distribution of a sequence $(x_1, \ldots, x_N)$
\begin{equation}
\label{eq:empirical_distribution}
\tilde{p}(x) := \sum_{n=1}^{N} \delta(x - x_n),
\end{equation}
and $p(x | \theta)$ be a model distribution. 

Typically if we want to estimate the parameter $\theta$ for a given data set we maximize the log-likelihood of the data
\begin{equation}
\ell(x | \theta) := \sum_{n=1}^{N} \log p(x_n | \theta).
\end{equation}
Using KL divergence it is intuitive to select a $\theta$ that minimizes the distance between the model distribution and the empirical distribution. In fact, it turns out that both are equivalent:
\begin{eqnarray}
\KL{\tilde{p}(x)}{p(x | \theta)} &=& \int \tilde{p}(x) \log \frac{\tilde{p}(x)}{p(x | \theta)} dx \\
&=& - H(\tilde{p}(x)) - \int \tilde{p}(x) \log p(x | \theta) dx,
\end{eqnarray}
where $H(\tilde{p}(x)) =  \int \tilde{p}(x) \log \tilde{p}(x) dx $ is the entropy of $\tilde{p}(x)$. Note that the entropy is independent of the choice of $\theta$. Thus
\begin{equation}
\arg \min_{\theta} \KL{\tilde{p}(x)}{p(x | \theta)} = \arg \max_{\theta} \E_{\tilde{p}} \log p(x | \theta).
\end{equation}

Plugging \eqref{eq:empirical_distribution} into the right hand side gives
\begin{eqnarray}
\E_{\tilde{p}} \log p(x | \theta) &=& \frac{1}{T} \int \sum_{n=1}^{N} N \delta(x - x_n) \log p(x | \theta) dx \\
&=& \frac{1}{N} \sum_{n=1}^{N} \log p(x_n | \theta) \\
&=& \frac{1}{N} \ell(x | \theta)
\end{eqnarray}

Given this relation we can now evaluate the log-likelihood of $x$ given the KL divergence and entropy of the empirical distribution as
\begin{eqnarray}
\KL{\tilde{p}(x)}{p(x | \theta)} &=& - H(\tilde{p}) - \frac{1}{N} \ell(x | \theta) \\
\Leftrightarrow \ell(x | \theta) &=& -N \cdot \left(\KL{\tilde{p}(x)}{p(x | \theta)} + H(\tilde{p}) \right)
\end{eqnarray}

Since we can view the empirical spectrum as a multinomial probability mass function on the unit circle, the Kullback-Leibler divergence seems to be a natural candidate. The KL divergence between two discrete probability distribution $p_1, \ldots, p_K$ and $q_1, \ldots, q_K$ is defined as.
\begin{equation}
\KL{p}{q} := \sum_{i=1}^{K} p_i \logtwo \frac{p_i}{q_i}  = \E_p \logtwo \frac{p_i}{q_i}.
\end{equation}
Note however, that in general KL divergence is not symmetric: $\KL{p}{q} \neq \KL{q}{p}$. This violates the conditions needed for a proper application of Laplacian graphs and diffusion maps. A typical ``trick'' is to symmetrize KL divergence as 
\begin{equation}
\symKL{p}{q} := \frac{\KL{p}{q} + \KL{q}{p}}{2}.
\end{equation}

Hence for $\mathbf{X} = \left( s_{1}, \ldots, s_{n} \right) \in \R^{T \times n}$ the similarity matrix between spike $s_{i}$ and $s_{j}$ can be defined as
\begin{equation}
\mathbf{S} = \symKL{I(s_i)}{I(s_j)},
\end{equation}
where $I(s_k)$ is the periodogram estimate of spike $s_{k,t}$.

\begin{comment}

\section{Progress report}
For the project proposal I set the following ``milestones'':
\begin{itemize}
\item have an automated procedure that can succesfully extract the actual spikes (only noise remains)
\item characterize spikes theoretically and empirically so well that I can get useful features as a basis for classification.
\item Have a good idea about what a good (parametric) distribution fits the data/features; the raw data is obviously non-Gaussian; it might be possible to approximate the features  by (mixtures of) Gaussians.
\item Present preliminary results based on the models I have by then.
\end{itemize}

I think I have accomplished that mostly; maybe in the second point I don't have any highly theoretical characterizations, but the slowness measure seems to be a very reasonable feature that approaches the problem at its heart.
\end{comment}
